# Supplementary material for: Volume-optimal persistence homological scaffolds of hemodynamic networks covary with MEG theta-alpha aperiodic dynamics
Source: arXiv:2407.05060 ancillary file (2024-07-23)
Supplement: Supplementary file 1 [file Supplementary.pdf]

## Supplementary information

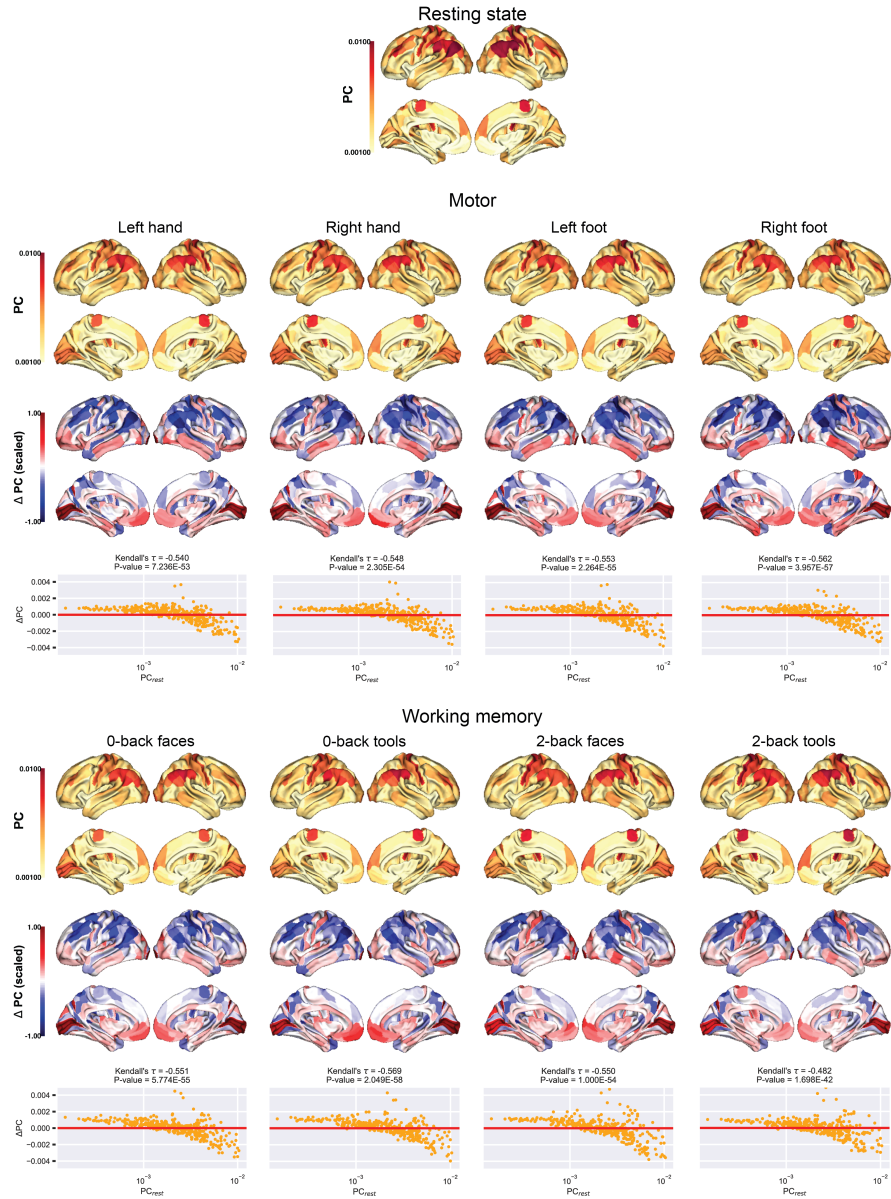

**Fig. 1.** Distributions of  $PC$  and  $\Delta PC$  of all task conditions, with scatter plots showing the correlations between  $PC_{rest}$  and  $\Delta PCs$ .

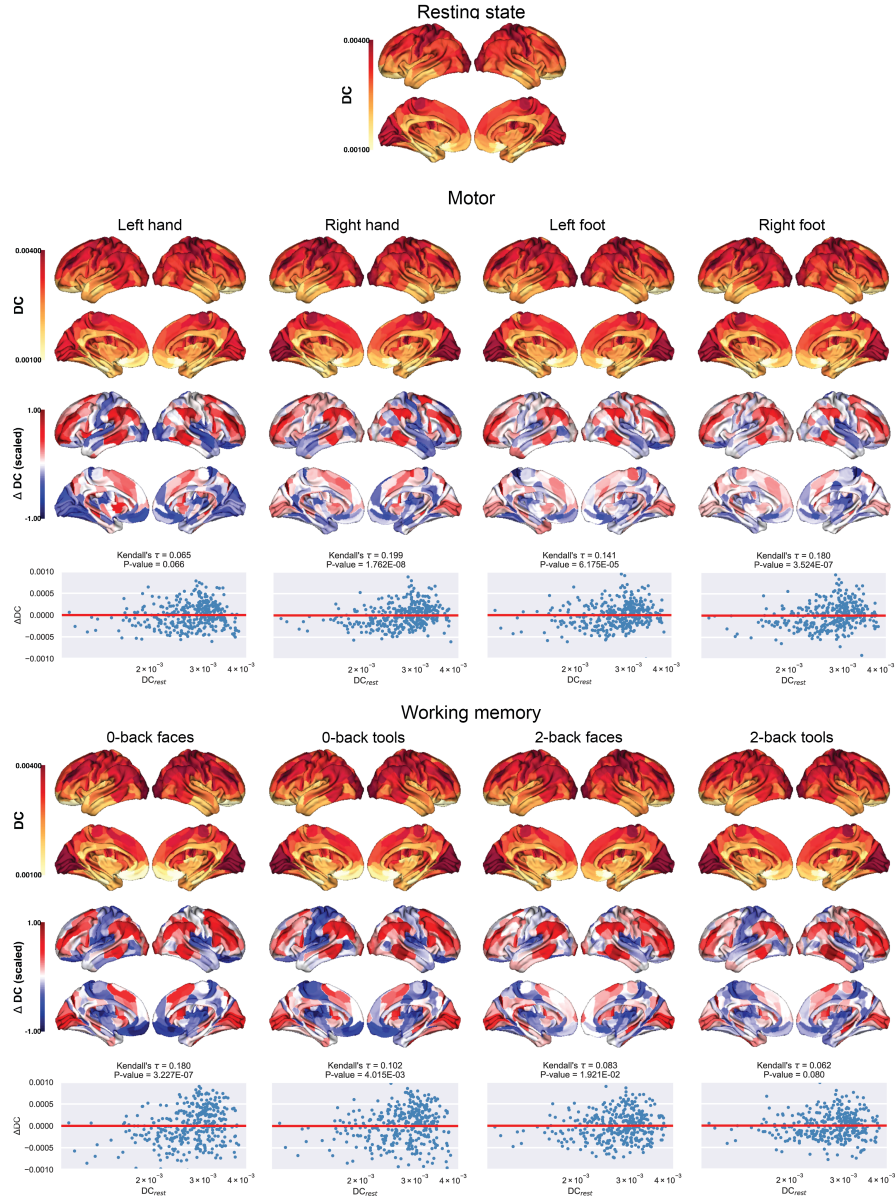

**Fig. 2.** Distributions of  $DC$  and  $\Delta DC$  of all task conditions, with scatter plots showing the correlations (or the lack thereof) between  $PC_{rest}$  and  $\Delta PC$ s.
